# Supplementary material for: Leveraging Instruction Tuning and Merging for Reasoning Model Adaptation
Source: arXiv:2607.14895 source file (2026-10-01)
Supplement: Supplementary file 3 [file app_prompts.tex]

\section{Prompts}
\label{app:prompt}

\lstdefinestyle{conversation-turn}{
    language={},
    keywordstyle=\ttfamily,
    commentstyle=\ttfamily,
    basicstyle=\ttfamily\scriptsize,
    breaklines=true,
    breakatwhitespace=false,
    breakautoindent=false,
    breakindent=10pt,
    columns=fullflexible,
    numbers=none,
    frame=none,
    xleftmargin=0pt,
    framexleftmargin=0pt,
    numbersep=0pt,
    escapeinside={(*@}{@*)},
    mathescape=true,
    showstringspaces=false
}

We use one task prompt for Rust code generation, one task prompt for text summarization, and four judge prompts for the text summarization evaluation.
\Cref{prompt:rust-code-generation} shows the Rust prompt used for both IFT training and MBPP Rust evaluation.
\Cref{prompt:text-summarization} shows the text summarization prompt used for both IFT training on the TLDR split and evaluation on the CNN split.
For the LLM-based text summarization metrics, Gemini 3 Pro is prompted separately for each criterion: \cref{prompt:relevance-evaluation} for relevance, \cref{prompt:fluency-evaluation} for fluency, \cref{prompt:consistency-evaluation} for factual consistency, and \cref{prompt:coherence-evaluation} for coherence.
In this section, we detail all prompts used for the respective models and tasks.
